# Supplementary material for: Bridging the Sim-to-Real Gap with Bayesian Inference
Source: arXiv:2403.16644 source file (2024-09-01)
Supplement: Supplementary file 1 [file appendix_dump.tex]

\section{Background}

\subsection{Definitions}

\begin{itemize}
    \item Input domain $\calX \subseteq \R^{d_\calX}$
    \item Target domain $\calY \subseteq \R^{d_\calY}$
    \item $\calM(A)$ Set of probability measures defined over the set $A$
\end{itemize}

\subsection{Variational Bayesian Neural Networks}

Input: 
\begin{itemize}
    \item Neural network architecture with parameter space $\Theta \subseteq \R^{d_\Theta}$ such that $\forall \theta \in \Theta$, $h_\theta: \calX \mapsto \calY$ defines a neural network map
    \item Prior probability distribution $p(\theta) \in \calM(\Theta)$
    \item Likelihood function $p(y|f(x)) \in \calM(\calY)$
    \item Variational family of posterior distributions $\calF := \{q_\phi(\theta) | \phi \in \Phi \} \subset \calM(\Theta)$. Often chosen as Gaussians with diagonal covariance matrix.
    \item Dataset $\calD = (\bX, \bY) = \{(x_i, y_i) \}_{i=1}^n$
\end{itemize}

Minimization Objective (negative ELBO):

\begin{align}
    \calL(\phi) &= - \E_{\theta \sim q_\phi} \left[ \log p(\bY| \bX, \theta) \right] + \text{KL} \left[q(\theta) || p(\theta) \right]  \\ 
    &=\E_{\theta \sim q_\phi} \left[ - \sum_{i=1}^n \log p(y_i, h_\theta(x_i)) + \log q(\theta) - \log p(\theta) \right] 
\end{align}

\subsection{Functional Variational BNNs}

Input: 
\begin{itemize}
    \item Neural network architecture with parameter space $\Theta \subseteq \R^{d_\Theta}$ such that $\forall \theta \in \Theta$, $h_\theta: \calX \mapsto \calY$ defines a neural network map
    \item Likelihood function $p(y|f(x)) \in \calM(\calY)$
    \item Variational family of posterior distributions $\calF := \{q_\phi(\theta) | \phi \in \Phi \} \subset \calM(\Theta)$. Often chosen as Gaussians with diagonal covariance matrix.
    \item Dataset $\calD = (\bX_\calD, \bY_\calD) = \{(x_i, y_i) \}_{i=1}^n$
    \item Stochastic process prior $p(f)$ with finite marginals $p(\bff^\bX) = p(f(x_1), ..., f(x_k))$
    \item Sampling distribution for measurement sets $s(x) \in \calM(\calX)$
\end{itemize}

Minimization Objective (negative fELBO):

\begin{align}
    \calL(\phi) &= - \E_{\theta \sim q_\phi} \left[ \log p(\bY| \bX, \theta) \right] + \E_{\bX^M \sim c} \left[ \text{KL} \left[q(\bh_\theta^\bX) || p(\bff^\bX) \right] \right] ~~, \text{where} ~~ \bX := [\bX^\calD, \bX^M ] \\ 
    &=\E_{\theta \sim q_\phi} \left[ - \sum_{i=1}^n \log p(y_i, h_\theta(x_i)) + \E_{\bX^M \sim c} \left[ \log q(\bh_\theta^\bX) - \log p(\bff^\bX) \right] \right]
\end{align}

\section{Score Estimation}

\subsection{Spectral Stein Gradient Estimator}

Goal: Approximate the score $\nabla_\bx \log p(\bx)$ of a probability distribution $p(\bx) \in \calM(\calX), ~ \calX \subseteq \R^d$ based on i.i.d samples $\bX = [\bx_1, ..., \bx_l, ..., \bx_m],~ \bx_l \sim p(\bx)$.

We denote the target score function as $\bg: \calX \mapsto \R^d(\bx): \bg(\bx) = \nabla_\bx \log p(\bx)$. The i-th component of the score is $g_i(\bx) = \frac{\partial}{\partial x_i} \log p(\bx)$. We assume that $g_1, ..., g_d \in L^2(\calX, p)$ are square-integrable functions w.r.t. the probability measure $p$.

\paragraph{Nystöm method}
Given a kernel $k(\bx, \bx')$, let $\{\psi_j\}_{j \geq 1}, \psi_j \in L^2(\calX, p)$ denote the eigenfunctions of $k(\bx, \bx')$ w.r.t. the probability measure $p$, i.e., $\forall j \geq 1$ there exists an eigenvalue $\mu_j$ such that
\begin{equation}
    \int k(\bx, \bx') \psi_j(\bx') p(\bx') d\bx' = \mu_j \psi_j(\bx) \;. \label{eq:eigenfun}
\end{equation}
In addition, the eigenfunctions $\{\psi_j\}_{j \geq 1}$ are orthonormal under $p$, i.e.
\begin{equation}
 \int \psi_i(\bx) \psi_j(\bx) d\bx = \delta_{i,j}. = \mathbf{1}[i=j] \;.
\end{equation}
If we approximate the LHS of (\ref{eq:eigenfun}) by $m$ i.i.d. Monte Carlo samples $\bX = [\bx_1, ..., \bx_m]$ from $p$, we obtain the eigenvector equation
\begin{equation}
    \frac{1}{m} \bK \boldsymbol{\psi} = \mu \boldsymbol{\psi} \;, \label{eq:eigenvector}
\end{equation}
where $\bK \in \R^{m \times m}$ is the kernel matrix $\bK_{ij} = k(\bx_i, \bx_j)$, $\boldsymbol{\psi} = [\phi(\bx_1), ..., \phi(\bx_m) ]^\top$ and $\mu \in \R$. Natuarlly, the solutions of (\ref{eq:eigenvector}) are the eigenvectors and corresponding eigenvalues of $\bK$. We sort the eigenvalues $\lambda_j$ in ascending order, i.e. $\lambda_1 \geq ... \geq \lambda_m$ and denote the corresponding eigenvectors as $\bu_j \in \R^m$.
Using the {\em Nystöm method} \citep{nystroem1930, baker1977}, we approximate the $j$-th eigenfunction as
\begin{equation}
    \psi_j(\bx) \approx \hat{\psi}_j(\bx) = \frac{\sqrt{m}}{\lambda_j} \sum_{l=1}^m u_{jl}k(\bx, \bx_l) \quad, ~ 1 \leq l \leq m
\end{equation}
wherein $u_{jl}$ is the $l$-th entry of the $j$-th eigenvector.

\paragraph{Approximating the score function}

Since $\{\psi_j\}_{j \geq 1}$ forms an eigenbasis of $L^2(\calX, p)$, we can expand $g_i(\bx)$ as spectral series:
\begin{equation}
    g_i(\bx) = \sum_{j=1}^\infty \beta_{ij} \psi_j(\bx) \;. \label{eq:spectral_expansion_g}
\end{equation}
Using Stein's identity, \citet{shi2018spectral} show that $\beta_{ij}$ can be approximated as
\begin{equation}
    \hat{\beta}_{i,j} = - \frac{1}{m} \sum_{l=1}^m \frac{\partial}{\partial x_i} \hat{\psi}_j(\bx_l) ;.
\end{equation}
Finally, the SSGE score estimator is obtained by substituting for emmpirical approximations $\hat{\psi}_j(\bx)$ and $\hat{\beta}_{i,j}$ into (\ref{eq:spectral_expansion_g}) and truncating the sum to the $J \leq m$ largest eigenvalues:
\begin{equation}
    \hat{\bg_i} (\bx) = \sum_{j=1}^J \hat{\beta}_{i,j} \psi_j(\bx) ;.
\end{equation}
As a heuristic for choosieng $J$, \citet{shi2018spectral} suggest a set a threshold $\bar{r}$ for the percentage of remaining eigenvalues and choose
\begin{equation}
    J = \argmax_{J'} \frac{\sum_{j'=1}^{J'} \lambda_{j'}}{\sum_{j=1}^m \lambda_{j}} \quad \text{s.t.} ~~ \frac{\sum_{j'=1}^{J'} \lambda_{j'}}{\sum_{j=1}^m \lambda_{j}} < \bar{r}
\end{equation}

\begin{algorithm}[t]
 \hspace*{\algorithmicindent} \textbf{Input:} i.i.d. samples $\bS = \{\bx_1, ..., \bx_m\}$ from $p(x)$ and query points $\bX = \{\bx_1, ..., \bx_k\}$\\
 \hspace*{\algorithmicindent} \textbf{Input:} kernel function $k(\bx, \bx')$ and eigenvalue coverage threshold $\bar{r}$ \\
 \hspace*{\algorithmicindent} \textbf{Return:} $\{ \hat{\bg}(\bx_1, ..., \hat{\bg}(\bx_k) \}$
\begin{algorithmic}[1]
\State Construct kernel matrix $\bK$ of the sample points $\bS$
\State $\{(\bu_j, \lambda_j)\}_{j=1}^m \leftarrow $ EigenvalueDecomposition($\bK$)
\State $J \leftarrow \max_{J'} \left\{ J' ~ \text{s.t.} \left(\sum_{j'=1}^{J'} \lambda_{j'} \right) / \left(\sum_{j=1}^m \lambda_{j} \right) < \bar{r} \right\}$
% \State $\hat{\psi}_j(\bx) = \frac{m}{\lambda_j} \sum_{l=1}^m u_{jl}k(\bx, \bx^m) \quad, ~ 1 \leq j \leq m$
\State $\bU \leftarrow [\bu_1, ..., \bu_j]~,~~ \boldsymbol{\Lambda} \leftarrow \text{diag}(\lambda_1, ..., \lambda_J)$
\State $- \frac{1}{\sqrt{m}} \boldsymbol{\Lambda} \bU^\top \bK \mathbf{1}$
\end{algorithmic}
\caption{SSGE($\bS$, $\bX$) \label{algo:ssge}}
\end{algorithm}

\subsection{Nonparametric Score Estimation}

\begin{itemize}
    \item $\calK$: matrix valued kernel $\calK: \calX \times \calX \rightarrow \R^{d \times d}$
    \item $\calH_\calK$: vector-valued RKHS induced by $\calK$
    \item sampling operator $S_\bx:  \calH_\calK \times \R^{Mq}$ and it's adjoint $S_\bx^*$
    \item integral operator $L_{\calK} f := \int_{\calX} \calK_{\bx} f(\bx) d\rho$
    \item empirical estimate of the integral operator: $\hat{L}_{\calK} f = \frac{1}{M} \sum_{m=1}^M \calK_{\bx^m} f(\bx^m) =\frac{1}{M} S^*_\bx S_\bx = \frac{1}{M} S^*_\bx \by$
\end{itemize}

The approach to score estimation:
\begin{equation} \label{eq:score_estima_as_regr}
    \hat{\bs}_{p,\lambda} = \argmin_{\bs \in \calH_\calK} \frac{1}{M}\sum_{m=1}^M \|\bs(\bx^m) - \bs_p(\bx^m)\|_2^2  + \frac{\lambda}{2}\|\bs\|^2_{\calH_{\calK}}.
\end{equation}
The general solution to (\ref{eq:score_estima_as_regr}) is
\begin{equation}
    \hat{\bs}^g_{p,\lambda} := g_\lambda(\hat{L}_{\calK}) \hat{L}_{\calK} s_p
\end{equation}
where $g_\lambda(\hat{L}_{\calK})$ is some form of pseudo-inverse of the empirical integral operator. In the case of Tikhonov regularization $g_\lambda(\hat{L}_{\calK}) = (\hat{L}_{\calK} + \lambda I)^{-1}$. 

Under mild regularity conditions, we have that
\begin{equation}
    L_{\calK} \bs_p = \E_\rho \left[ \calK_\bx \nabla \log p(\bx) \right] =  - \E_\rho \left[ \divgers{\bx} \calK_\bx^\top \right]
\end{equation}
and it's empirical counterpart
\begin{equation}
    \hat{\zeta} := - \frac{1}{M} \sum_{m=1}^M \divgers{\bx} \calK_\bx^\top 
\end{equation}
Thus, the general score estimator follows as:
\begin{equation}
    \hat{\bs}^g_{p,\lambda} := g_\lambda(\hat{L}_{\calK}) \hat{\zeta}
\end{equation}

\paragraph{Curl-free kernels}
Score vector fields are gradient fields. We can use curl-free kernels \citep{fuselier2007refined, macedo2010learning} to capture this property. We can construct a curl-free matrix-valued kernel from the negative Hessian of a translation-invariant kernel $k(\bx, \bx') = \phi(\bx - \bx')$: 
\begin{equation}
    \calK_{\mathrm{cf}}(\bx, \bx') := - \nabla^2 \phi(\bx - \bx')
\end{equation}
If we construct curl-free kernels from an isotropic kernel $k(\bx, \bx') = \phi(\norm{\bx - \bx'})$ where $\br = (\bx - \bx')^\top$ and $r = \norm{\br}$, then the curl-free kernel follows as \citep{zhou2020nonparametric}:
\begin{equation}
    \calK_{\mathrm{cf}}(\bx, \bx') = \left( \frac{\phi'}{r^3} - \frac{\phi''}{r^2} \right)\br \br'^\top - \frac{\phi'}{r} \mathbf{I}.
\end{equation}
and its divergence as
\begin{equation}
    \divgers{\bx} \calK_{\mathrm{cf}}(\bx, \bx') = - \frac{\br}{r} \left[ \phi'''(r) + \frac{d-1}{r} \left(\phi''(r) - \frac{\phi'(r)}{r} \right)\right] ~.
\end{equation} 
In the special case of $\calK_{\mathrm{cf}}(\bx, \bx') := - \nabla^2 \rho(\norm{\bx - \bx'}^2)$, we recover
\begin{align}
        \calK_{\mathrm{cf}}(\bx, \bx') =& - 4 \rho'' \br \br'^\top - 2\rho' \mathbf{I} \\
        \divgers{\bx} \calK_{\mathrm{cf}}(\bx, \bx') = & - 4 \left[ \left( d + 2 \right) \rho'' + 2 r^2 \rho''' \right] \br
\end{align}

\paragraph{$\nu$-Method \citep{engl1996regularization}}
The $\nu$-method solves the inverse problem $g_\lambda(\hat{L}_{\calK})$ via the following fix-point iteration
\begin{align}
      \hat \bs_{p}^{(0)} &= 0,  \quad 
     \hat \bs_{p}^{(1)} = -\omega_1 \hat{\boldsymbol{\zeta}},  \\
     \hat \bs_{p}^{(t)} &= \hat \bs_{p}^{(t-1)}
        + u_t(\hat \bs_p^{(t-1)} - \hat \bs_p^{(t-2)})
        + \omega_t(-\hat{\boldsymbol{\zeta}} - \hat L_\calK \hat \bs_p^{(t-1)}) \\
        &= a_t \boldsymbol{\zeta} + \mathbf{K}_{\bx\bX} \bc_t
\end{align}
where $u_t$ and $\omega_t$ are given by the following polynomials
\begin{align}
    u_t &= \frac{(t-1)(2t-3)(2t+2\nu-1)}{(t+2\nu-1)(2t+4\nu-1)(2t+2\nu-3)},\\
    \omega_t &= \frac{4(2t+2\nu-1)(t+\nu-1)}{(t+2\nu-1)(2t+4\nu-1)}.
\end{align}
and $a_t$, $\bc_t$ are recursively defined defined through
\begin{align}
     a_t &:= (1 + u_t)a_{t-1} - u_ta_{t-2} - \omega_t, \\
       \bc_t &:=(1+u_t)\bc_{t-1}
        - \frac{\omega_t}{M}(a_{t-1}\bh + \bK\bc_{t-1})
        - u_t \bc_{t-2},
\end{align} with 
$\bc_0 = \bc_1 = 0$, $a_0 = 0$, $a_1 = -\omega_1$ and $\bh = (\hat{\zeta}(\bx_1), ..., \hat{\zeta}(\bx_m)) \in \R^{Md}$.
